# Supplementary material for: StarryGazer: Leveraging Monocular Depth Estimation Models for Domain-Agnostic Single Depth Image Completion
Source: arXiv:2512.13147 source file (2025-12-15)
Supplement: Supplementary file 1 [file supp_list.tex]

% SILog Metric 수식 추가

% Rendered Handpose 내용 옮기기
% Rendered handpose dataset에서 MDE model Global, Segment affine transform 결과 측정
% Rendered handpose dataset 그림 수정 (배경의 depth값 날리고, hand에 해당하는 depth값으로 colormap 수정해보기, 지금은 hand는 완전 푸른색 단색으로 나와서 문제됨)
% ClearGrasp와 Rendered handpose에서 iMAE나 iRMSE 뽑을 수 있나? supple에 표 만드면 나쁘지 않을듯

% Model Agnosticism across MDE models에 DepthAnythingV2와 비교했는데 (Table S4), 우리가 main paper에서 비교했던 Metric3D나 Unidepth로 비교해 볼 수 있나? Depthanything v2와 비교한 결과는 큰 의미가 없을거 같아서

% Segment-wise affine transform과 StarryGazer(Ours)에서 Segment-wise SILog average 구할 수 있나? global SILog하고 같이 비교해서 설명할 수 있으면 좋을듯

% (정말 시간되면) ICCV Reviewer3가 이야기했던 dataset 하나 더 실험 추가

----
